# Supplementary material for: Approximate Bayesian inference in spatial environments
Source: arXiv:1805.07206 source file (2019-06-20)
Supplement: Supplementary file 1 [file appendix.tex]

\documentclass[conference]{IEEEtran}
\usepackage{times}
\usepackage{multicol}

\usepackage[numbers]{natbib}

\usepackage[utf8]{inputenc} %
\usepackage[T1]{fontenc}    %
\usepackage{breakcites}
\usepackage[bookmarks=true]{hyperref}       %
\usepackage{url}            %
\usepackage{booktabs}       %
\usepackage{amsfonts}       %
\usepackage{nicefrac}       %
\usepackage{microtype}      %

\usepackage{amsmath}
\usepackage{amssymb}
\usepackage{makecell}
\usepackage{todonotes}
\usepackage{graphicx}
\usepackage{cleveref}
\usepackage{siunitx}
\usepackage{subcaption}
\usepackage{wrapfig}
\usepackage{graphicx}
\usepackage{tikz}
\usepackage{algpseudocode,algorithm,algorithmicx}
\usepackage{mymath}
\usepackage{mlmacros}

\usetikzlibrary{positioning,shapes,arrows}

\variables{z,x,u,m,y}
\probdists{p,q}
\probdists[dirac]{\delta}

\newcommand{\showappendix}{1}       %
\newcommand{\ifappendix}[1]{\ifthenelse{\equal{\showappendix}{1}}{#1}{}}

\crefname{appsec}{appendix}{appendices}

\pdfinfo{
   /Author (Homer Simpson)
   /Title  (Robots: Our new overlords)
   /CreationDate (D:20101201120000)
   /Subject (Robots)
   /Keywords (Robots;Overlords)
}

\begin{document}

\title{Approximate Bayesian inference in spatial environments - Appendix}
\author{Author Names Omitted for Anonymous Review.}
\maketitle

\IEEEpeerreviewmaketitle

\ifappendix{
    \newpage
    \appendices
    \crefalias{section}{appsec}
    \input{appendices/dvbflm.tex}
    \input{appendices/navigation.tex}
    \input{appendices/exploration.tex}
    \input{appendices/lossobstacle.tex}
    \input{appendices/pema.tex}
    \bibliographystyle{plainnat}
    \bibliography{related}
}

\end{document}
